# Supplementary material for: Diffusion Lens: Interpreting Text Encoders in Text-to-Image Pipelines
Source: arXiv:2403.05846 source file (2024-10-21)
Supplement: Supplementary file 1 [file additional_results.tex]

\section{Additional Results}
\ho{TODO decide how this should be merged into the paper}
\paragraph{Mix of concepts}
\citet{rassin2022dalle}, depicted concepts that can be interpreted in more than one way, such as a bat, which can be viewed as both an animal and a tool, and often ends up in images that contain both. Here we see a similar pattern in the early layers. Earlier layers tend to have

\paragraph{First layers}
The 7 first layers in Deep Floyd look very different from the later layers, although many times, the patterns correspond to the prompt that exists in the images, especially colors. We believe that our method fails to generate coherent images from these layers due to a big gap in the distribution of the weights in their layers. Future work might look into this phenomenon and try to find a method that would work on these layers. 
In Stable Diffusion 2.1 we see a similar pattern, although these images are less colorful. The five first layers have different textures. The images in later layers look more similar to regular images.
