# Supplementary material for: Diffusion Lens: Interpreting Text Encoders in Text-to-Image Pipelines
Source: arXiv:2403.05846 source file (2024-10-21)
Supplement: Supplementary file 2 [file 7.appendix-old.tex]

\section{Appendix}
\label{sec:appendix}



\subsection{Prompts}
\label{sec:appendix:prompts}
The full list of prompts can be found in the git, together with the images dataset and annotations.

\subsection{Annotation}
\label{sec:appendix:prompts}
The following section demonstrated the annotation questions in detail as was shown to the annotators.

General question:
Good Quality - does the image have a good quality? (compared to the very last layer (23/24))

Color experiment:
First Color Wrong/Second Color Wrong - does the first/second color (by order in the sentence) appear on the other object, or in an unnatural place in the image, such as background etc.
Please provide an answer concerning the major color of the object/animal.
First Color Correct/Second Color Correct - does the first/second color (by order in the sentence) appear on the correct object (as a major color)?

Common/Uncommon Animals:
Is Animal - Is there any animal in the image? (Not including humans)
Is Mammal - If there is an animal, does it look like a mammal? I.e. hairy, no wings, etc. (Not including human)
Same Fur - If there is an animal, does it have the same fur as an image from the internet?
Same Face - If there is an animal, does it have the same face with an image from the internet?

Relations:
First Thing Exists - does the first thing exist in the image?
Second Thing Exists - does the second thing exist in the image?
Relation Correct - does the relation is correct in the image?

Famous People:
Is Human - Is there a human in the image?
Same Gender - If there is a human, is he/she from the same gender?
Same Style - Does the style of clothing is similar to the famous person?
Same Face - Does the fame look like the real person?
 

\subsection{Stable Diffusion Plots}
\label{fig:stable_diffusion_plots}
